# Supplementary material for: Analyzing and Mitigating Data Stalls in DNN Training
Source: arXiv:2007.06775 source file (2021-01-19)
Supplement: Supplementary file 1 [file fig-analysis-batch.tex]

\begin{figure}[!t]
  \centering 
   \includegraphics[width=.44\textwidth]{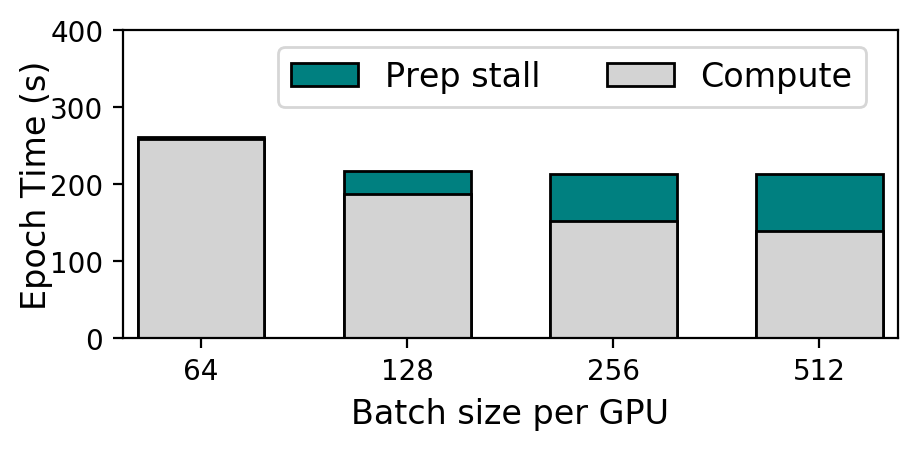}
  
  \mycaption{Impact of batch size on prep}{This graph plots the epoch time for MobileNetv2 on \confssd with 8-GPUs as we vary the per-GPU batch size. As batch size increases, the compute time at the GPU drops due to reduced communication overhead. However, the epoch time does not improve because training is bottlenecked by prep.}
  \vspace{-1mm}
  \label{fig-analysis-batch}

\end{figure}
