# Supplementary material for: Analyzing and Mitigating Data Stalls in DNN Training
Source: arXiv:2007.06775 source file (2021-01-19)
Supplement: Supplementary file 2 [file fig-tool.tex]

\begin{figure}[!t]

  {\includegraphics[width=0.48\textwidth]{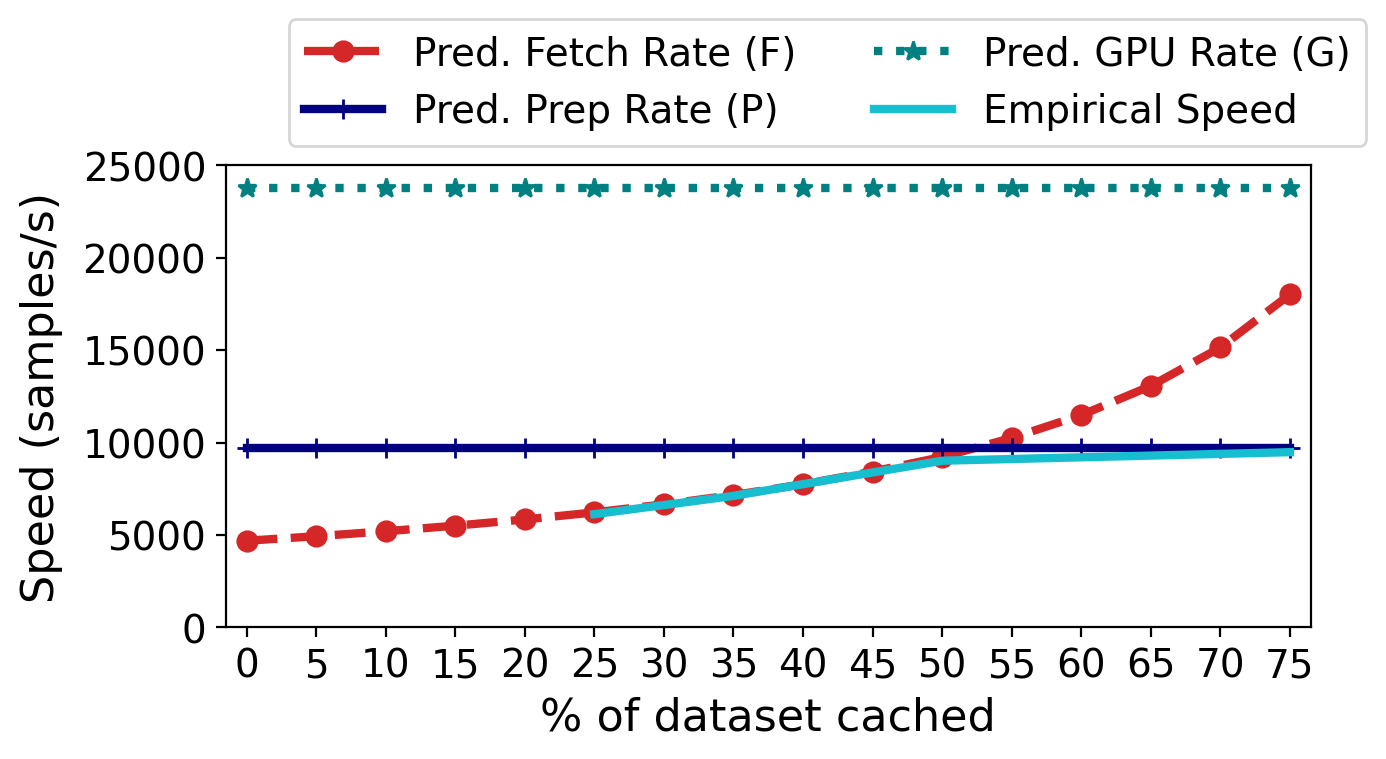}}
   
  \mycaption{Estimating optimal cache size with \tool}{ }
  \label{fig-tool-cache}
  \vspace{-4mm}
\end{figure}
