# Supplementary material for: Analyzing and Mitigating Data Stalls in DNN Training
Source: arXiv:2007.06775 source file (2021-01-19)
Supplement: Supplementary file 3 [file fig-analysis-cache-dist.tex]

\begin{figure}[!t]
  \centering 
   \includegraphics[width=.45\textwidth]{graphs-dali/analysis-cache-dist.png}
  
  \caption{Distributed training across servers with 35\% cache on each server}
  \vspace{-1mm}
  \label{fig-analysis-cache-dist}

\end{figure}
