# Supplementary material for: Analyzing and Mitigating Data Stalls in DNN Training
Source: arXiv:2007.06775 source file (2021-01-19)
Supplement: Supplementary file 4 [file fig-analysis-cache-hp.tex]

\begin{figure}[!t]
  \centering 
   \includegraphics[width=.45\textwidth]{graphs-dali/analysis-cache-hp.png}
  
  \caption{HP search on a server with 35\% cache}
  \vspace{-1mm}
  \label{fig-analysis-cache-hp}

\end{figure}
