# Supplementary material for: Analyzing and Mitigating Data Stalls in DNN Training
Source: arXiv:2007.06775 source file (2021-01-19)
Supplement: Supplementary file 5 [file fig-analysis-cache-models.tex]

\begin{figure*}[!t]
  \centering 
   \includegraphics[width=.85\textwidth]{graphs-dali/analysis-cache-all.png}
  
  \caption{Impact of cache size on single server DNN training}
  \vspace{-1mm}
  \label{fig-analysis-cache-models}

\end{figure*}
