# Supplementary material for: Analyzing and Mitigating Data Stalls in DNN Training
Source: arXiv:2007.06775 source file (2021-01-19)
Supplement: Supplementary file 6 [file fig-analysis-cache.tex]

\begin{figure*}[!t]
  \centering 
   \includegraphics[width=.8\textwidth]{graphs-dali/analysis-cache.png}
  
  \mycaption{Impact of cache size on DNN training}{The percentage of
    dataset cached, heavily influences the throughput of DNN training,
    in a variety of training scenarios. When dataset resides on slower
    storage media like HDD (\confhdd), training can slowdown by 19\myx
    for Resnet18. On \confssd, smaller DNNs like ShuffleNet train upto
    2\myx slower when only 35\% of the dataset is cached.
  }
  \vspace{-1mm}
  \label{fig-analysis-cache}

\end{figure*}
