# Supplementary material for: Analyzing and Mitigating Data Stalls in DNN Training
Source: arXiv:2007.06775 source file (2021-01-19)
Supplement: Supplementary file 7 [file fig-analysis-fetch.tex]

\begin{comment}
\begin{figure*}[!tbh]
  \centering 

      \subfloat[Varying the datastore - Epoch 1\label{fig-analysis-store-ep1} ]{{\includegraphics[width=.3\linewidth, height = 3.4cm]{figures/analysis-store-ep1.pdf} }}
      \quad
      \subfloat[Varying the datastore - Steady state epoch\label{fig-analysis-store-ep3}]{{\includegraphics[width=.3\linewidth, height = 3.4cm]{figures/analysis-store-ep3.pdf} }}%  
      \quad
     \subfloat[GFS vs Blobfuse\label{fig-analysis-store-comp}]{{\includegraphics[width=.3\linewidth, height = 3.4cm]{figures/analysis-blob-vs-gfs.pdf} }}%  

     % \subfloat[Varying the cache size\label{fig-analysis-cache}]{{\includegraphics[width=.45\linewidth,height = 4.2cm]{figures/analysis-cache.pdf} }}%
        
     \mycaption{Impact of data store on DNN training}{The plot shows
       how per-epoch training time varies when different data stores
       are used for storing the dataset. }
  \label{fig-analysis-fetch-appendix}
\end{figure*}
\end{comment}

\begin{figure}[!t]
  \centering 
  \includegraphics[width=.45\textwidth]{graphs/analysis-blob-vs-gfs.pdf}
  \mycaption{Azure Blob vs GFS}{The plot shows the time to accuracy for ResNet18 on 8 GPUs. We analyze two data stores - Azure Blob and GlusterFS.}
  \label{fig-analysis-store-comp}
  \end{figure}
