# Supplementary material for: Analyzing and Mitigating Data Stalls in DNN Training
Source: arXiv:2007.06775 source file (2021-01-19)
Supplement: Supplementary file 8 [file fig-analysis-hyperparam.tex]

\begin{figure}[!t]
  \centering 
\includegraphics[width=.45\textwidth]{graphs-dali/analysis-hyperparam.pdf}

\mycaption{Varying the number of 1-GPU jobs per node}{The graph shows
  that as the number of jobs (ResNet18, 100\% cached) on a machine
  increases, data stalls increase, even if all the available cores are
  used for preprocessing.}
  \label{fig-analysis-hyperparam}
\end{figure}
