# Supplementary material for: Analyzing and Mitigating Data Stalls in DNN Training
Source: arXiv:2007.06775 source file (2021-01-19)
Supplement: Supplementary file 9 [file fig-analysis-prep-res18.tex]

\begin{figure*}[!t]
  \centering 
   \includegraphics[width=.95\textwidth]{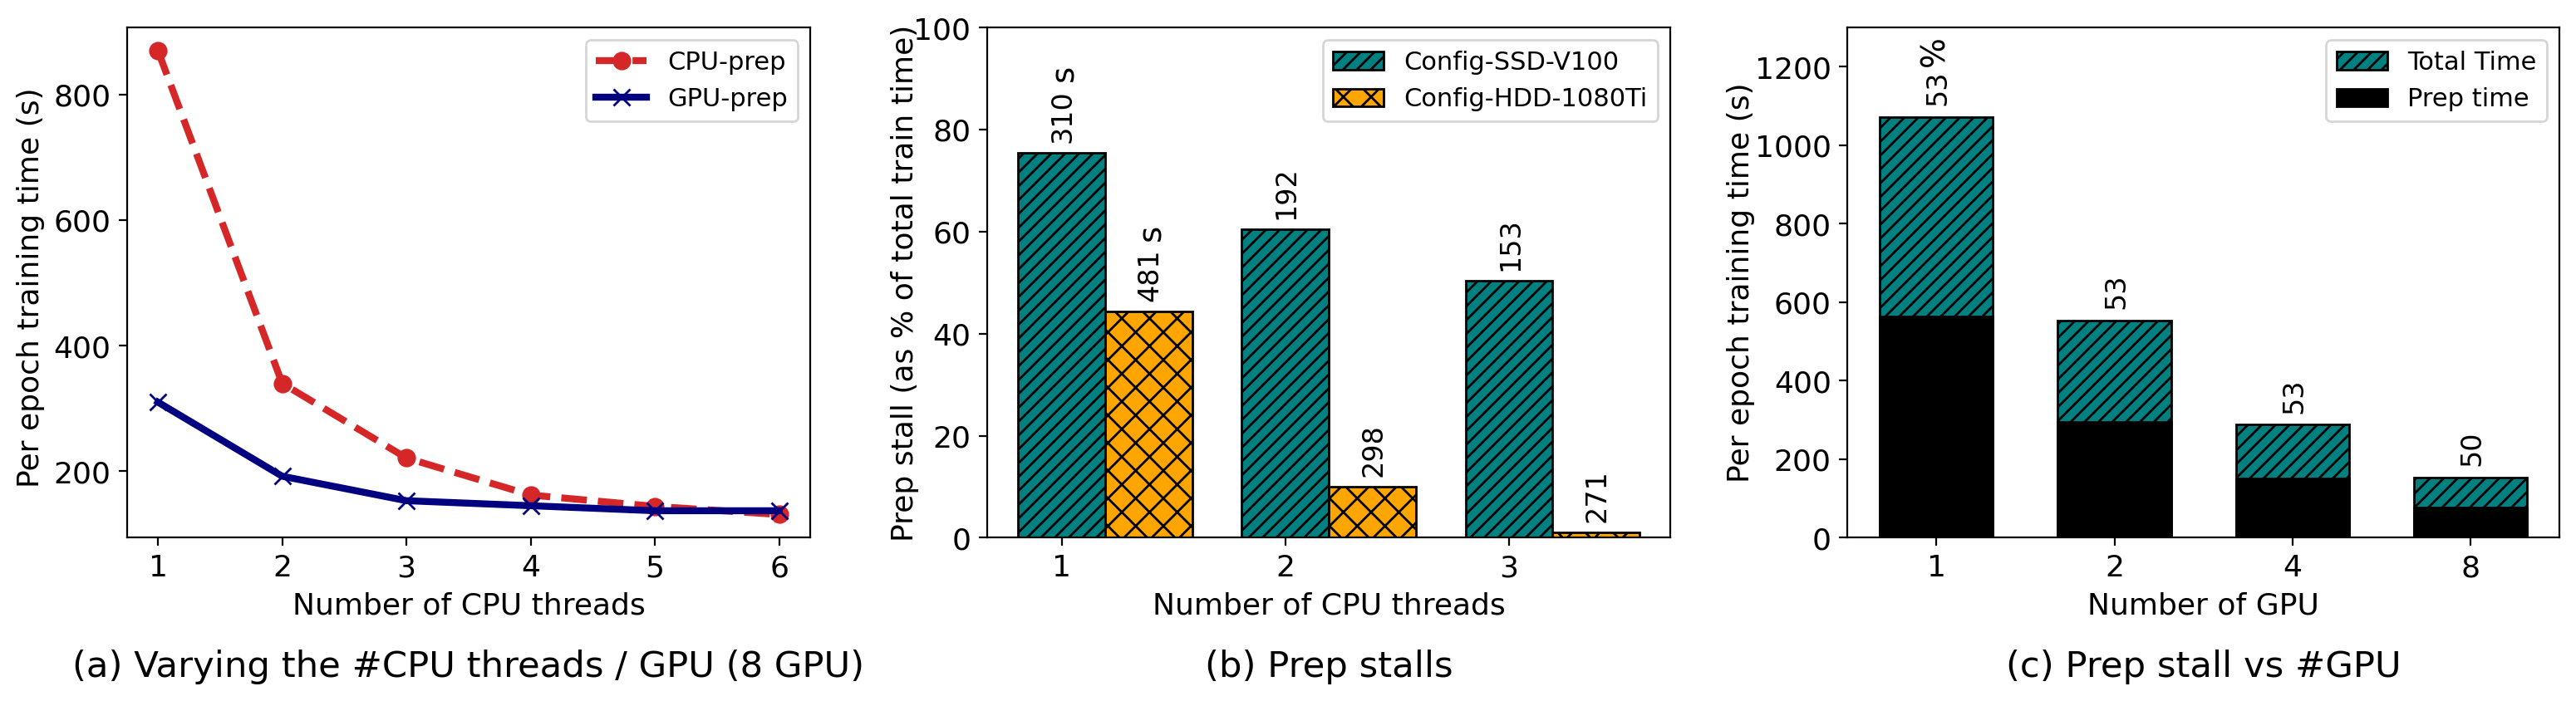}
  
  \caption{Multi-GPU ResNet18 training}
  \vspace{-1mm}
  \label{fig-analysis-prep-res18}

\end{figure*}
