# Supplementary material for: Analyzing and Mitigating Data Stalls in DNN Training
Source: arXiv:2007.06775 source file (2021-01-19)
Supplement: Supplementary file 10 [file fig-analysis-prep.tex]

\begin{figure*}[!h]
  \centering 
   \includegraphics[width=1\textwidth]{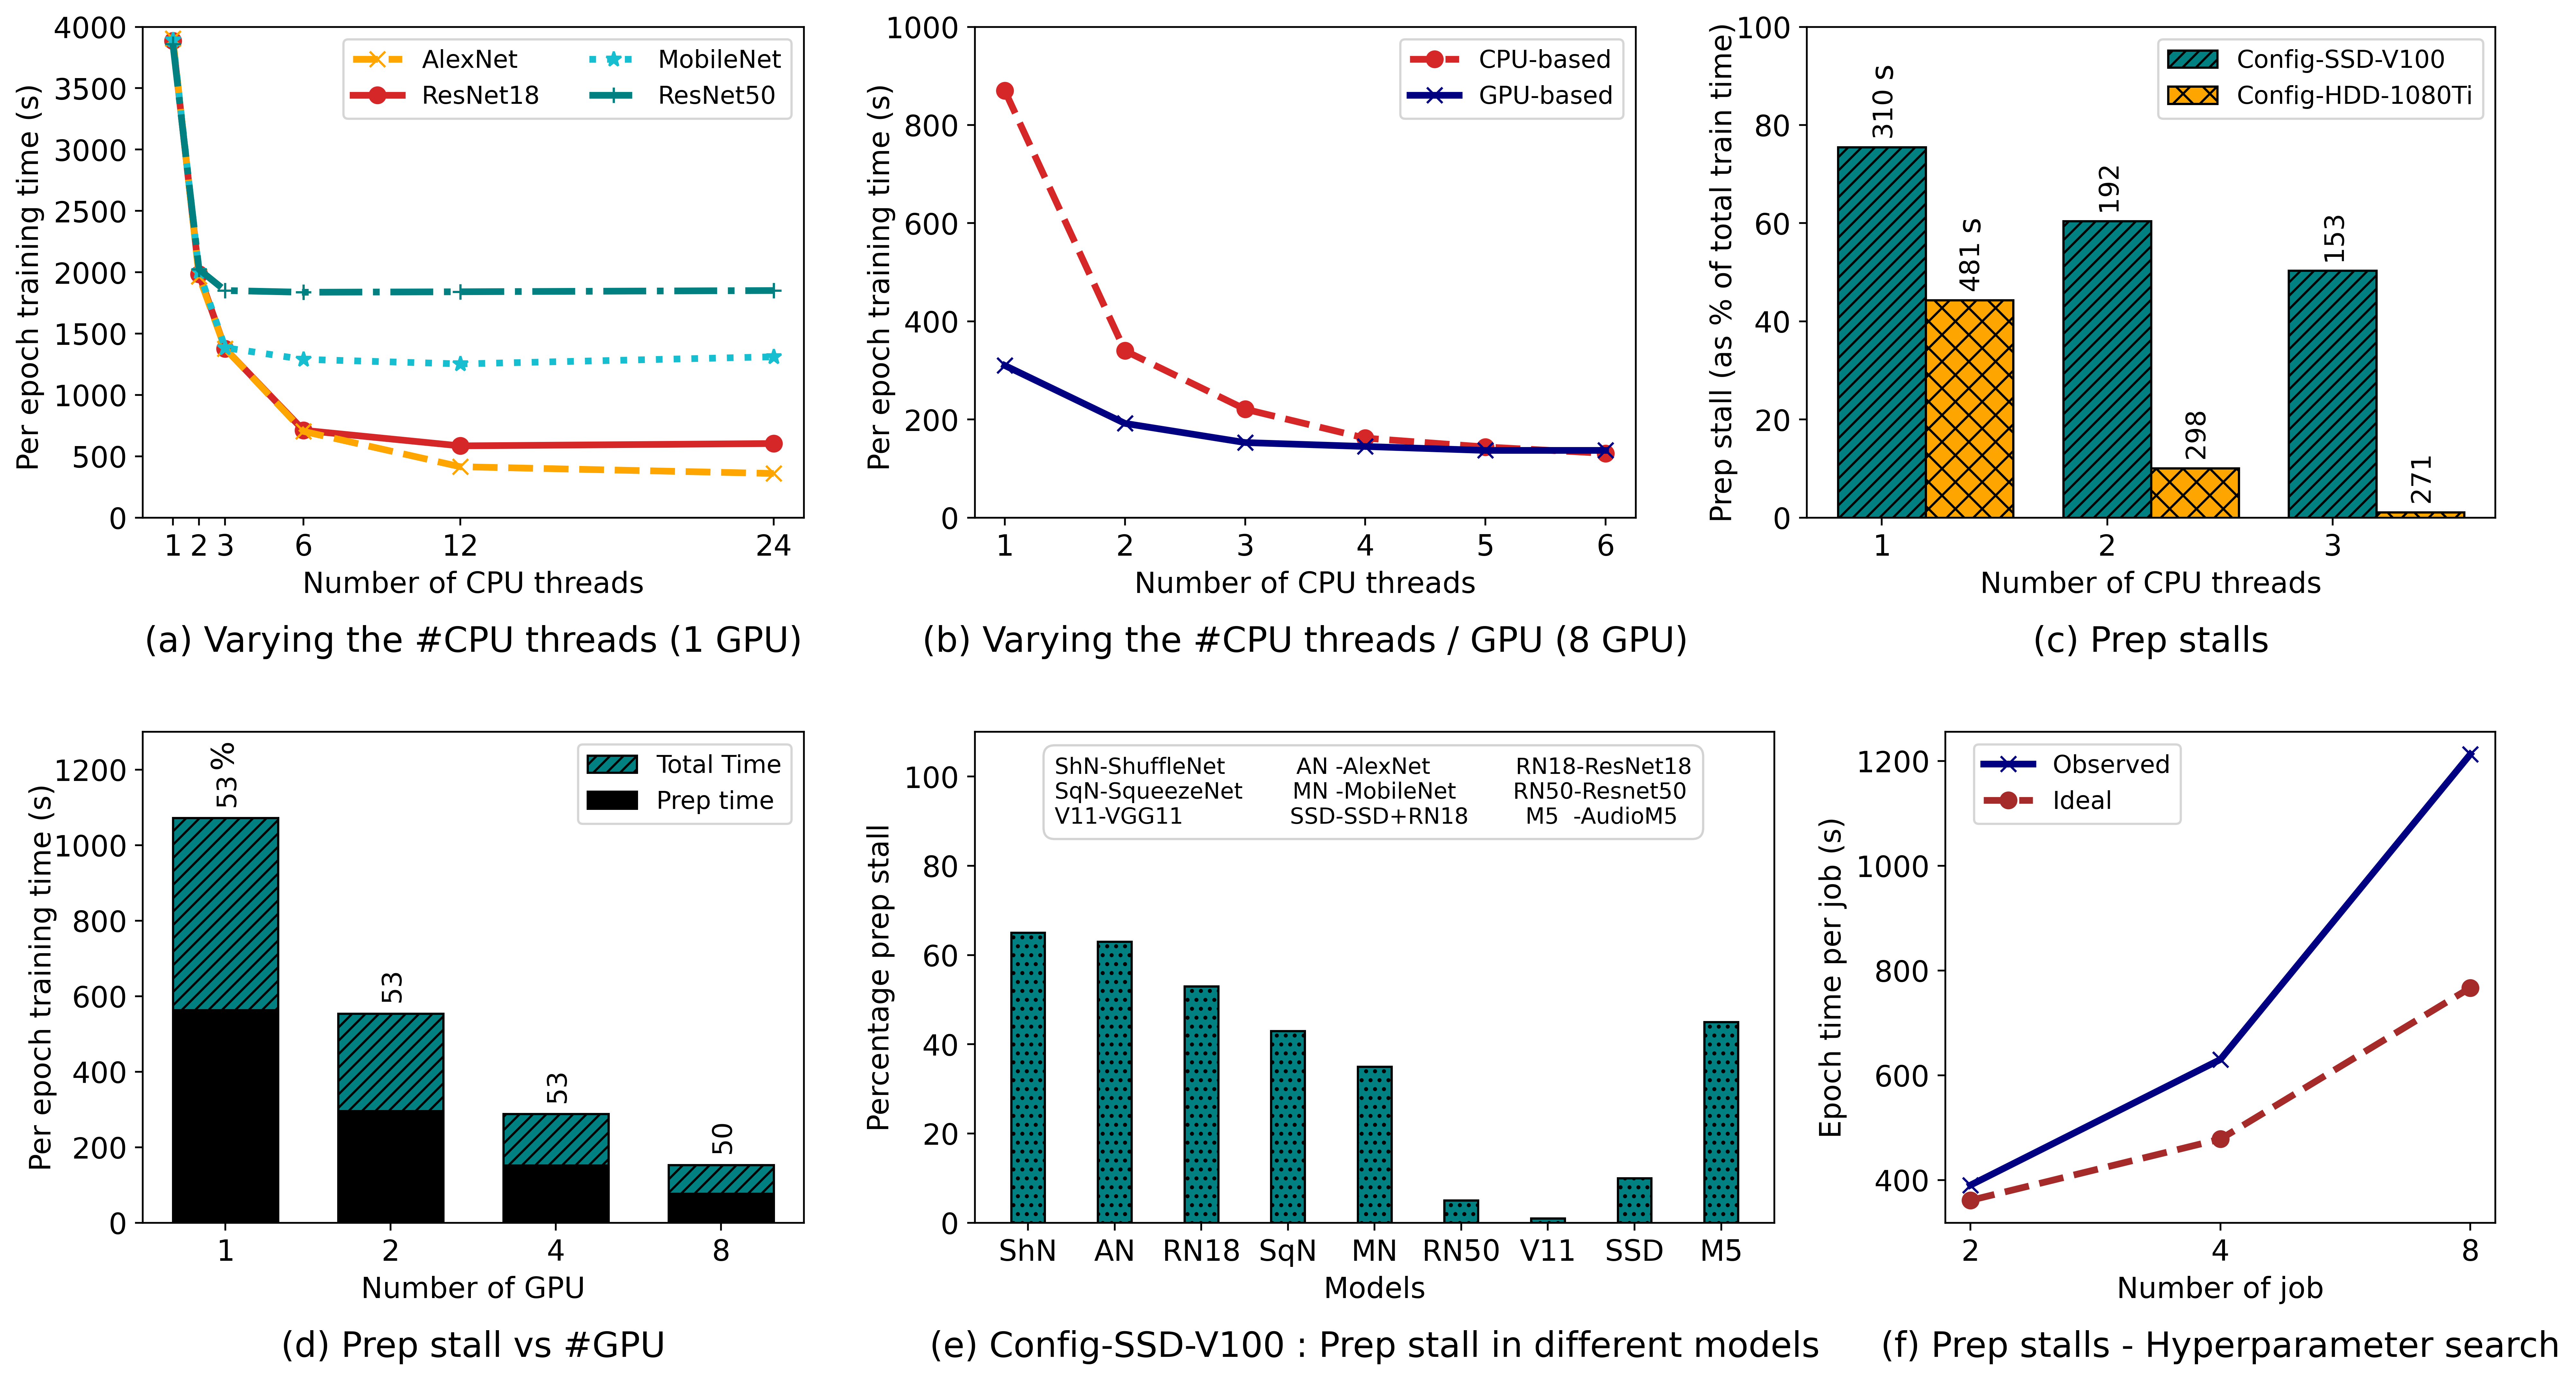}
  
  \mycaption{Impact of pre-processing on DNN training}{This graph shows the impact on prep stalls on DNN training
  time under various circumstances. Prep stalls are dominant across different models, and GPU generations. }

  \label{fig-analysis-prep}

\end{figure*}
