# Supplementary material for: Analyzing and Mitigating Data Stalls in DNN Training
Source: arXiv:2007.06775 source file (2021-01-19)
Supplement: Supplementary file 11 [file fig-analysis-preprocess-gpus.tex]

\begin{figure}[!t]

  \centering 
   
 % \subfloat[Varying the workload for 1 GPU job~\label{fig-analysis-1gpu}]{{\includegraphics[width=\linewidth, height = 5.5cm]{figures/analysis-workload-1gpu.pdf} }}
  
%   \subfloat[Varying the workload for 4 GPU job~\label{fig-analysis-4gpu}]{{\includegraphics[width=0.47\linewidth, height = 4.2cm]{figures/analysis-workload-4gpu.pdf} }}
%   \qquad
 %  \subfloat[Varying the workload for 8 GPU job~\label{fig-analysis-8gpu}]{{\includegraphics[width=0.47\linewidth, height = 4.2cm]{figures/analysis-workload-8gpu.pdf} }} 
  \includegraphics[width=0.47\textwidth, height=4.5cm]{graphs-dali/analysis-workload-line.pdf}
   \mycaption{Analysis of data stalls for various DNNs when the
     dataset is fully cached}{ The plot shows the impact of compute
     misses for 7 different DNNs when trained using 8 GPUs. The data pipeline cannot keep up
     with the ingest rate requirements, resulting in significant data
     stalls.}
     %The labels are read as;\\
    % \textbf{A}:AlexNet, \textbf{Sh}:ShuffleNet, \textbf{R18}:ResNet18, \textbf{Sq}:SqueezeNet, \textbf{M}:MobileNet, \textbf{R50}:ResNet50, \textbf{V}:VGG16}
  \label{fig-analysis-preprocess-gpus}
\end{figure}
