# Supplementary material for: Analyzing and Mitigating Data Stalls in DNN Training
Source: arXiv:2007.06775 source file (2021-01-19)
Supplement: Supplementary file 12 [file fig-analysis-preprocess.tex]

\begin{figure}[!tbh]

  \centering 
  %\subfloat[Varying the number of data workers\label{fig-analysis-workers}]{{\includegraphics[width=.3\linewidth, height = 3cm]{figures/analysis-workers.pdf} }}%
%\qquad

  \subfloat[Multi-GPU training\label{fig-analysis-num-gpu}]{{\includegraphics[width=.45\textwidth]{graphs-dali/analysis-num-gpu.pdf} }}%
  
    \subfloat[Data parallel training across 8 GPUs (varying the GPU generation and \# pre-processing threads)
  \label{fig-analysis-gpu}]{{\includegraphics[width=.45\textwidth]{graphs-dali/analysis-gpu.pdf} }}%
  \vspace{-3mm}
  \mycaption{Analysis of data stalls when the dataset is completely
     cached}{The plot shows the impact of compute misses
     (pre-processed data is not available in the cache) for a ResNet18
     training job under different scenarios. Even when the dataset is
     completely cached, pre-processing data leads to significant data
     stalls in many scenarios. Percentages represent data stall
     overheads (\% of total epoch time).}
  \label{fig-analysis-preprocess}

\end{figure}
