# Supplementary material for: Analyzing and Mitigating Data Stalls in DNN Training
Source: arXiv:2007.06775 source file (2021-01-19)
Supplement: Supplementary file 13 [file fig-cache-dist-mint.tex]

\begin{figure*}[!h]
  \centering 
    \subfloat[Distributed training across 32 GPUs\label{fig-analysis-cache-hdd}]{{\includegraphics[width=.45\textwidth, height=4cm]{graphs-dali/cache-dist-mint.png} }}%
  \qquad
  \subfloat[Dataset on SSD
  \label{fig-analysis-cache-ssd}]{{\includegraphics[width=.45\textwidth, height=4cm]{graphs-dali/hp-35cache.png} }}%
        \mycaption{Impact of cache size on DNN training}{As we vary the percentage of cached dataset for a ResNet training job running across 8 GPUs, training time is affected significantly. For hard disks, the training time increases by  29\myx if only 20\% of the dataset is cached (Y-axis is log scale), while for solid state drives, it increases by 25\%. }
        \vspace{-1mm}
  \label{fig-analysis-cache}

\end{figure*}
