# Supplementary material for: Analyzing and Mitigating Data Stalls in DNN Training
Source: arXiv:2007.06775 source file (2021-01-19)
Supplement: Supplementary file 14 [file fig-cache.tex]

\begin{figure}[!t]

  {\includegraphics[width=0.3\textwidth]{graphs/cache.pdf}}
   
  \caption{Architecture of \dl using \sysname}%{This figure shows the architecture of the modified PyTorch \dl using \sysname. Raw data items from the local or remote store are cached using the \mint policy to reduce store misses. Multiple data workers fetch items from this cache (or datastore), pre-process and collate them into minibatches, which are then staged for sharing across jobs. Similar DNN training jobs (accessing the same dataset) reuse minibatches in the \emph{batch cache}.}
  \label{fig-cache}
  \vspace{-4mm}
\end{figure}
