# Supplementary material for: Analyzing and Mitigating Data Stalls in DNN Training
Source: arXiv:2007.06775 source file (2021-01-19)
Supplement: Supplementary file 15 [file fig-data-pipeline.tex]

\begin{figure}[!t]
  \centering
  \includegraphics[width=0.47\textwidth]{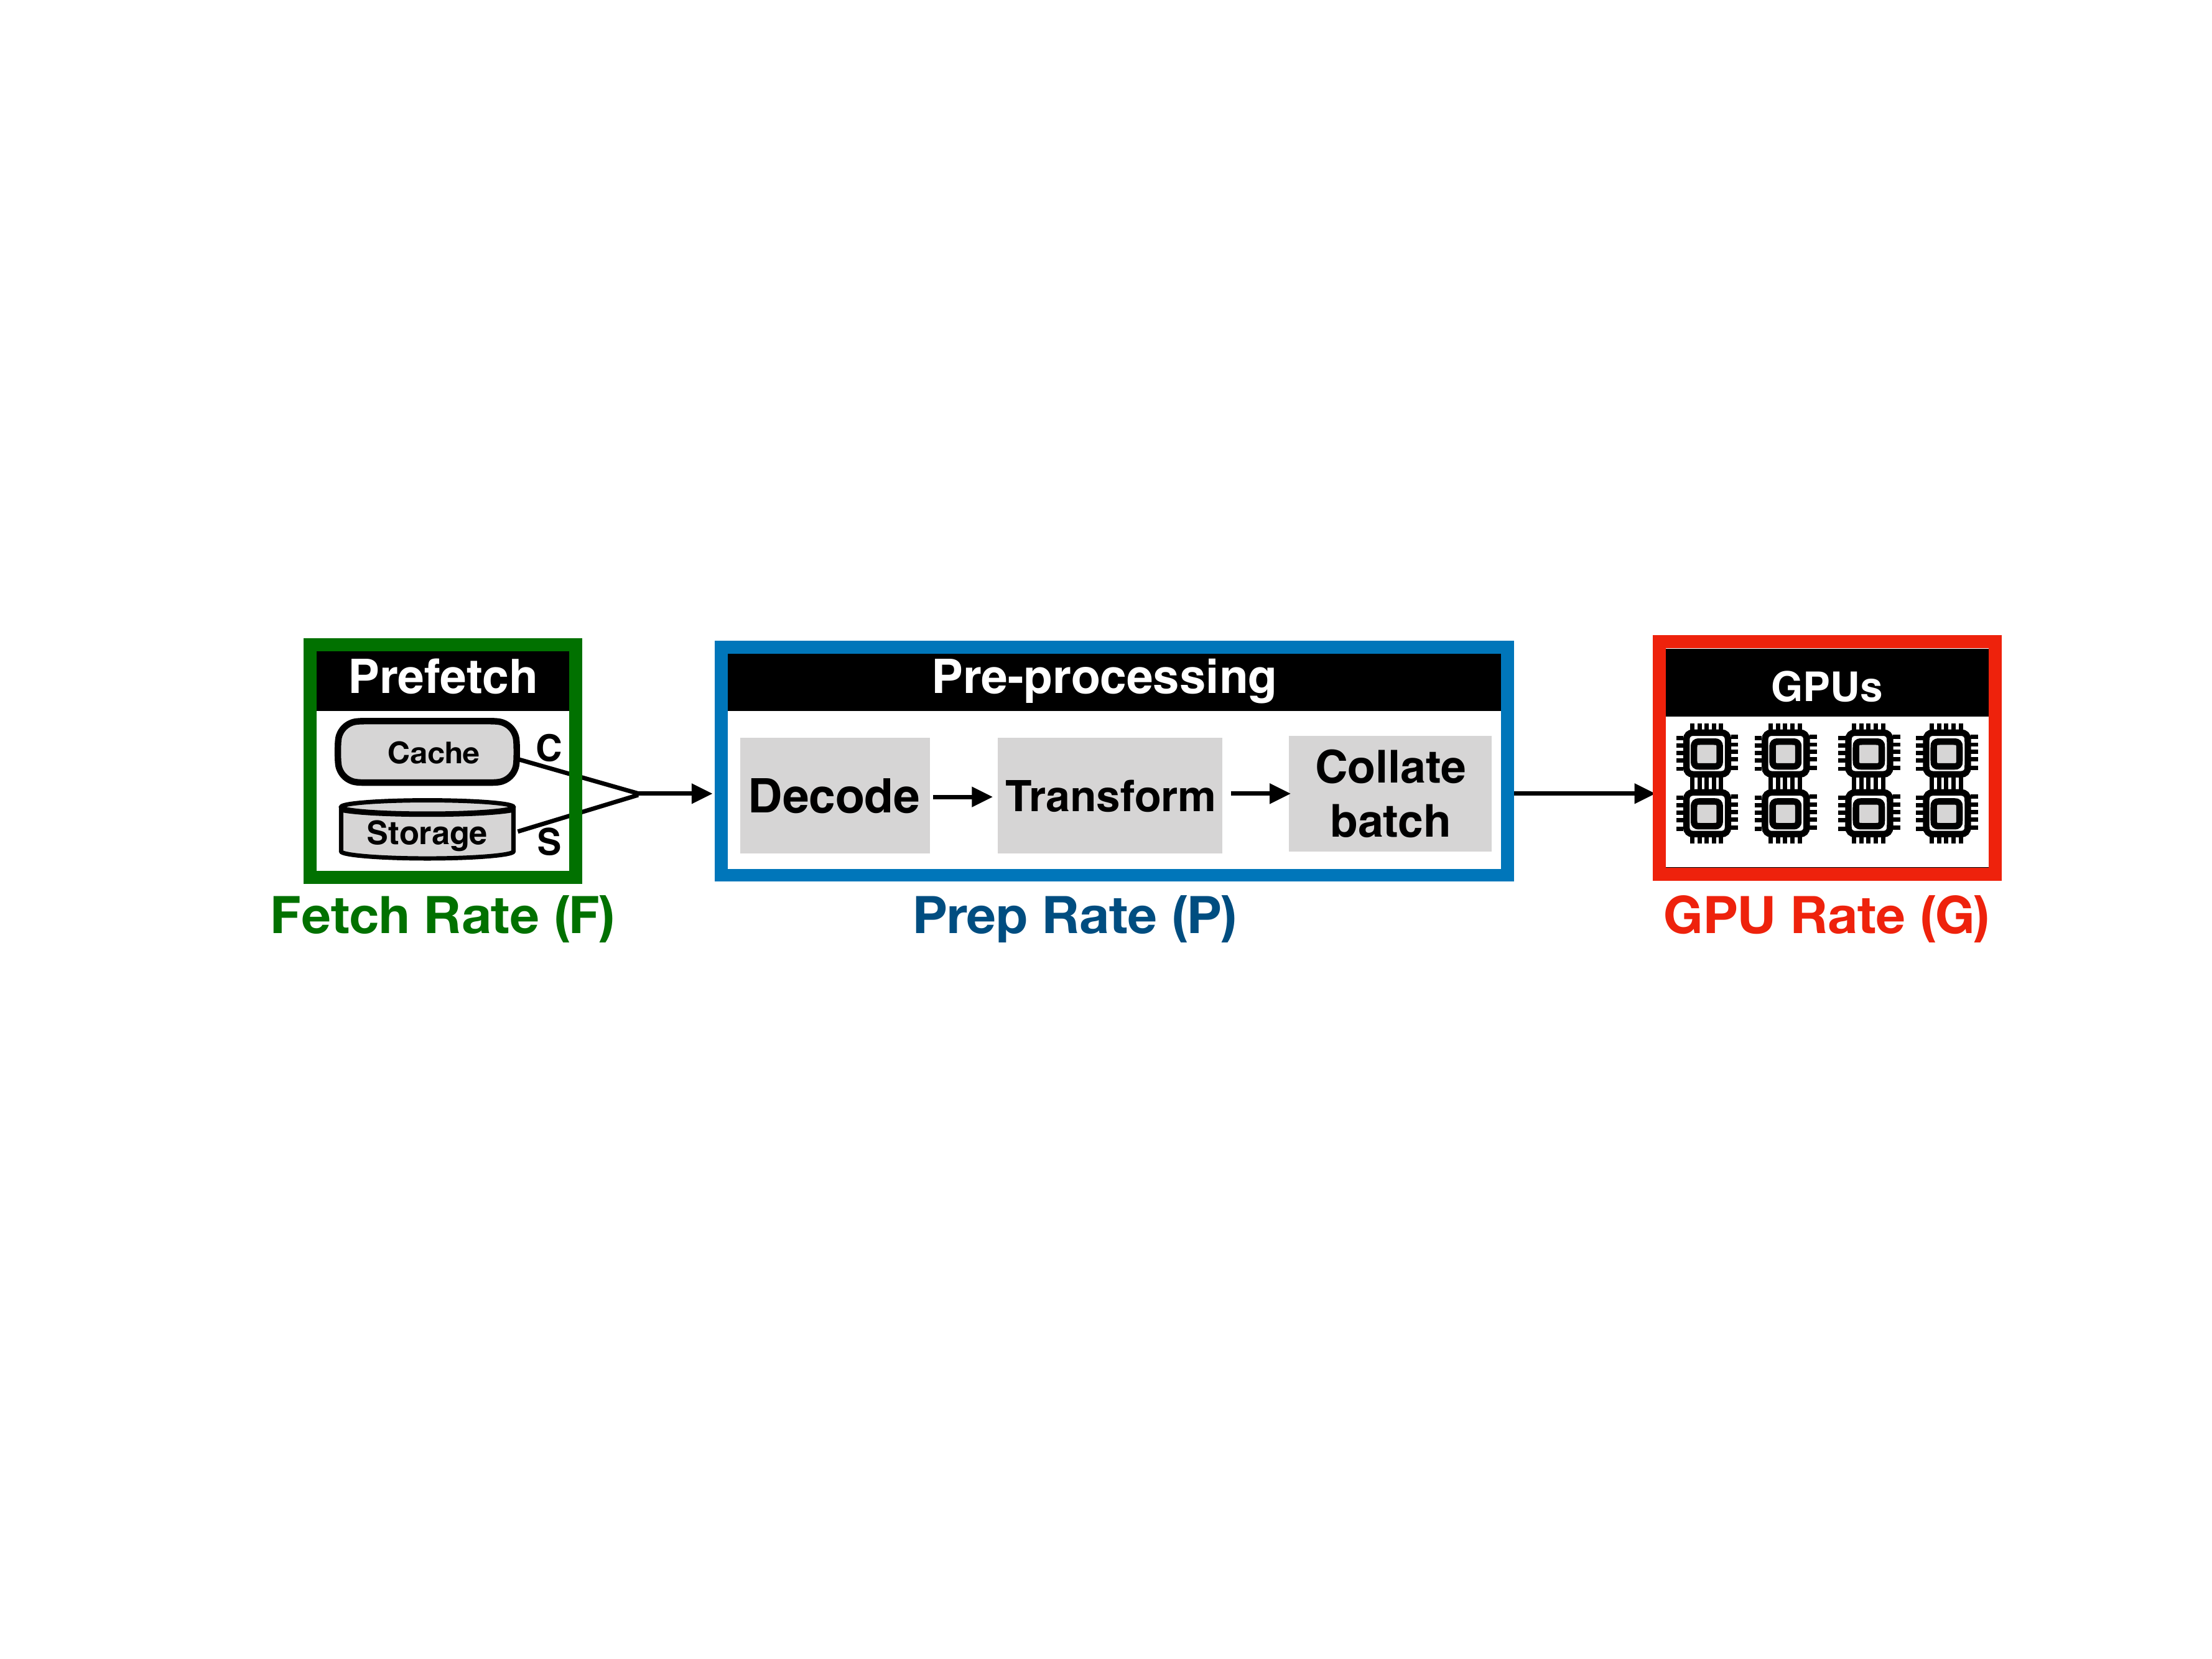}
  \mycaption{Data Pipeline in DNN Training}{This figure shows how
  data fetch and pre-processing at the CPU is pipelined with 
  GPU computation.  When GPU computes on a minibatch,
  several CPU threads fetch and pre-process minibatches 
  in parallel.\vc{not sure if this figure is adding value}}
    \vspace{-3mm}
  \label{fig-data-pipeline}
\end{figure}
