# Supplementary material for: Analyzing and Mitigating Data Stalls in DNN Training
Source: arXiv:2007.06775 source file (2021-01-19)
Supplement: Supplementary file 17 [file fig-eval-dist-mint.tex]

\begin{figure*}[!h]
  \vspace{-3mm}
  \centering 

 \subfloat[Alexnet-OpenImages\label{fig-analysis-cache-hdd}]{{\includegraphics[width=.3\textwidth, height=4cm]{graphs-dali/dist-mint-alexnet.png} }}%
\qquad
 \subfloat[ResNet50-OpenImages\label{fig-analysis-cache-hdd}]{{\includegraphics[width=.3\textwidth, height=4cm]{graphs-dali/dist-mint-res50.png} }}%
\qquad
 \subfloat[Audio-FMA\label{fig-analysis-cache-hdd}]{{\includegraphics[width=.3\textwidth, height=4cm]{graphs-dali/dist-mint-m5.png} }}%

    \mycaption{Evaluation of dist-mint caching}{The graphs compare the native PyTorch DataLoader with the modified DataLoader that uses \sysname's \mint caching policy.}
  \label{fig-eval-mcache}

\end{figure*}
