# Supplementary material for: Analyzing and Mitigating Data Stalls in DNN Training
Source: arXiv:2007.06775 source file (2021-01-19)
Supplement: Supplementary file 18 [file fig-eval-e2e.tex]

\begin{figure*}[!tbh]
  \centering 
    \vspace{-5mm}
      \subfloat[End-to-end workload on HDD\label{fig-e2e-hdd}] {{\includegraphics[width=.44\linewidth]{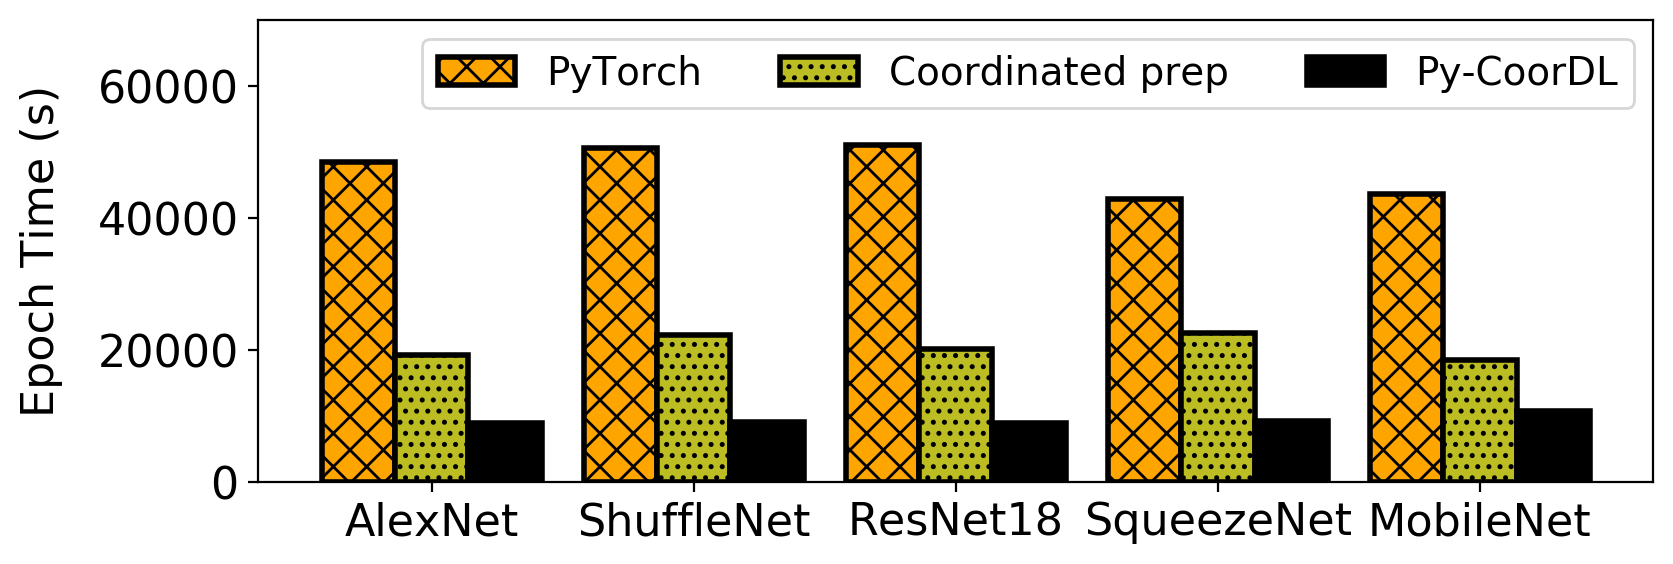} }}%
       \qquad
       \subfloat[End-to-end workload on SSD\label{fig-e2e-ssd}] {{\includegraphics[width=.44\linewidth]{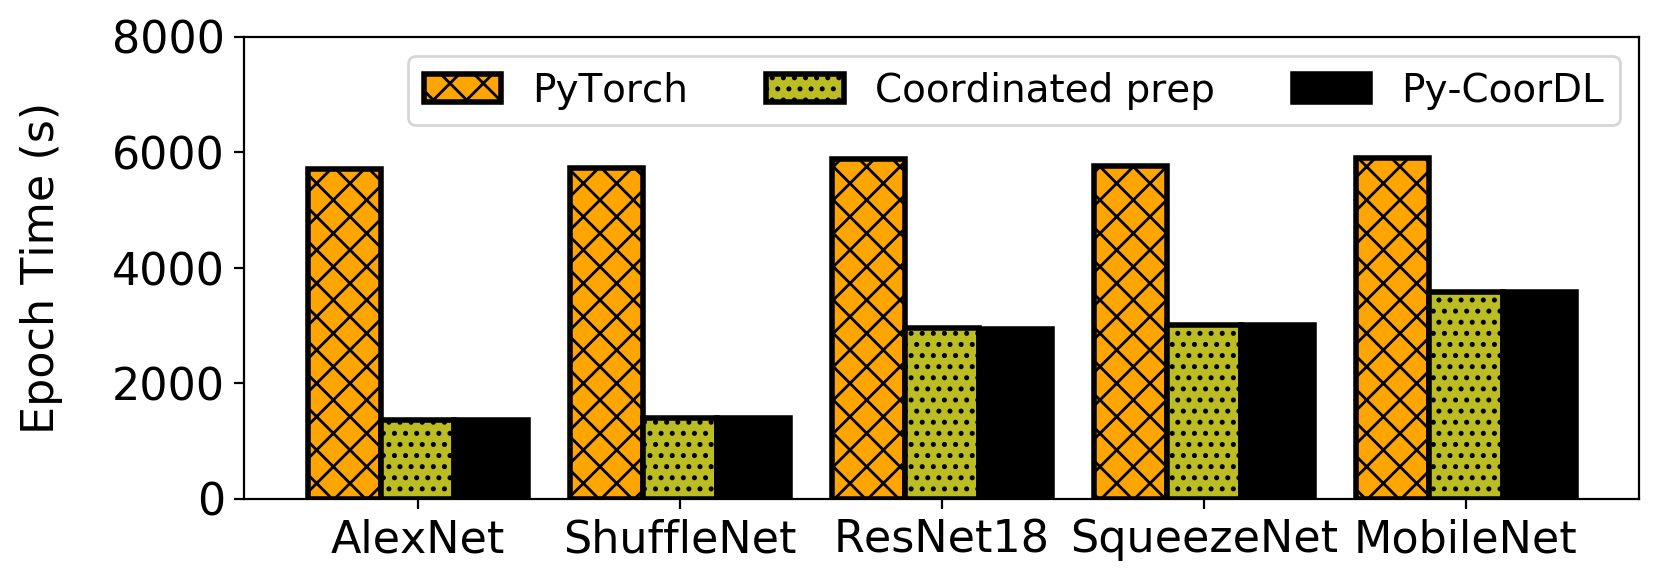} }}%
       \vspace{-3mm}       
         \mycaption{End-to-end evaluation}{The graphs compare the total search time for hyperparameter optimization using the baseline PyTorch \dl and \sysname on hard disks and solid state drives}
  \label{fig-eval-e2e}
  \vspace{-3mm}
\end{figure*}
