# Supplementary material for: Analyzing and Mitigating Data Stalls in DNN Training
Source: arXiv:2007.06775 source file (2021-01-19)
Supplement: Supplementary file 19 [file fig-eval-hp.tex]

\begin{figure*}[!h]
  \vspace{-3mm}
  \centering 

 \subfloat[Alexnet-HP vary jobs\label{fig-analysis-cache-hdd}]{{\includegraphics[width=.35\textwidth, height=4cm]{graphs-dali/hp-varyjobs.png} }}%
\qquad
 \subfloat[Hyperparameter search 8 jobs\label{fig-analysis-cache-hdd}]{{\includegraphics[width=.6\textwidth, height=4cm]{graphs-dali/eval-hp.png} }}%

    \mycaption{Hyperparameter search with \sysname}{The graphs compare the native PyTorch DataLoader with the modified DataLoader that uses \sysname's \mint caching policy.}
  \label{fig-eval-mcache}

\end{figure*}
