# Supplementary material for: Analyzing and Mitigating Data Stalls in DNN Training
Source: arXiv:2007.06775 source file (2021-01-19)
Supplement: Supplementary file 20 [file fig-eval-io-tbl.tex]

\begin{figure*}[!t]
\centering

	\begin{tabular}{l}
		\subfloat[Disk IO
		\label{tbl-dist-mint-io}]{
			  \ra{1.3}
  		 \begin{tabular}{lrrr}	 	
		\toprule[1pt]
		& \multicolumn{2}{c}{Speed(samples/s)}\\
		Model  & DALI & \sysname \\
		\midrule
		ShuffleNet & 1441 & 1.81\myx \\
		AlexNet & 1399 & 1.87\myx \\
		ResNet18 & 1056 & 1.53\myx \\
		SqueezeNet & 835 & 1.50\myx \\
		MobileNet & 752 & 1.35\myx \\
		ResNet50 & 569 & 1.21\myx \\
		VGG11 & 552 & 1.22\myx \\
		\bottomrule[1pt]
		\end{tabular}
		}%
		\quad
		\subfloat[Distributed training \label{fig-dist-mint-micro}]{\adjustbox{raise=-9.5pc}{\includegraphics[width=.75\textwidth]{graphs-dali/mint-resource.png}} }
		\label{fig-eval-dist-mint-micro}
	\end{tabular}

\end{figure*}
