# Supplementary material for: Analyzing and Mitigating Data Stalls in DNN Training
Source: arXiv:2007.06775 source file (2021-01-19)
Supplement: Supplementary file 21 [file fig-eval-mcache.tex]

\begin{figure*}[!h]
  \vspace{-3mm}
  \centering 

  \includegraphics[width=.9\linewidth, height=5cm]{graphs-dali/mint-sku1.png}

    \mycaption{Evaluation of \mint caching policy}{The graphs compare the native PyTorch DataLoader with the modified DataLoader that uses \sysname's \mint caching policy.}
  \label{fig-eval-mcache}

\end{figure*}
