# Supplementary material for: Analyzing and Mitigating Data Stalls in DNN Training
Source: arXiv:2007.06775 source file (2021-01-19)
Supplement: Supplementary file 22 [file fig-eval-ucache-mem.tex]

\begin{figure}[!t]
  \centering 
    \subfloat[Native \dl\label{fig-eval-mem-vanilla}]{{\includegraphics[width=.45\linewidth]{graphs/eval-mem-vanilla.pdf} }}%
    \quad
     \subfloat[With batch caching\label{fig-eval-mem-modified}]{{\includegraphics[width=.45\linewidth]{graphs/eval-mem-modified.pdf} }}%
    \mycaption{Memory footprint of batch caching}{The graphs compares memory footprint of the native PyTorch DataLoader with the modified DataLoader that uses \sysname's batch caching technique.}
    \vspace{-5mm}
\end{figure}
