# Supplementary material for: Analyzing and Mitigating Data Stalls in DNN Training
Source: arXiv:2007.06775 source file (2021-01-19)
Supplement: Supplementary file 23 [file fig-eval-ucache.tex]

\begin{comment}
 \begin{figure*}[!tbh]
  \centering 
  
    \subfloat[Compute misses\label{fig-compute-miss}]{{\includegraphics[width=.3\linewidth]{graphs/eval-compute-miss.pdf} }}%
    \quad
     \subfloat[Microbenchmark\label{fig-ucache-micro}]{{\includegraphics[width=.3\linewidth, height=3.3cm]{graphs/eval-unified-micro.pdf} }}%
   \quad
   \subfloat[Macrobenchmark- Ray Tune\label{fig-ucache-macro}]{{\includegraphics[width=.3\linewidth, height=3.3cm]{graphs/eval-unified-ray.pdf} }}%
  
      \mycaption{Evaluation of per-epoch batch caching}{The graphs compare vanilla dataloader in Pytorch with the modified dataloader that uses \sysname's batch caching technique.}
  \label{fig-eval-ucache}
\end{figure*}
\end{comment}

 \begin{figure*}[!tbh]
  \centering 
     \subfloat[Batch staging policy for SSD at 100\% cache\label{fig-ucache-100p}]{{\includegraphics[width=.4\linewidth]{graphs-dali/hp-micro-25p.pdf} }}%
  \quad
  \subfloat[Batch staging policy for SSD at 25\% cache\label{fig-ucache-25p}]{{\includegraphics[width=.4\linewidth]{graphs-dali/hp-micro-25p.pdf} }}%
   \mycaption{Evaluation of per-epoch batch caching}{Compares PyTorch against \sysname's  batch caching.}
    \label{fig-ucache-micro}
    \vspace{-4mm}
\end{figure*}
