# Supplementary material for: Analyzing and Mitigating Data Stalls in DNN Training
Source: arXiv:2007.06775 source file (2021-01-19)
Supplement: Supplementary file 24 [file fig-mint-resource.tex]

\begin{figure*}[!t]
\centering
  {\includegraphics[width=0.85\textwidth]{graphs-dali/mint-resource.png}}
   
  \mycaption{I/O and CPU utilization with \mint}{This plot shows the disk I/O access pattern, and the CPU utilization over time for DALI and \sysname when training ResNet18 on OpenImages. DALI gets cache hits at the start of every epoch; however due to thrashing, all requests result in disk access beyond a point. \sysname has a uniform disk access pattern by eliminating thrashing; this reflects in the predictable CPU I/O wait time. \sysname reduces CPU I/O wait, thereby using available CPU effectively for useful pre-processing.}
  \label{fig-mint-res}
  \vspace{-4mm}
\end{figure*}
