# Supplementary material for: Analyzing and Mitigating Data Stalls in DNN Training
Source: arXiv:2007.06775 source file (2021-01-19)
Supplement: Supplementary file 25 [file fig-motivation.tex]

\begin{figure}[!t]
  %{\includegraphics[width=0.95\textwidth]{figures/motivation.pdf}}
  {\includegraphics[width=0.47\textwidth]{graphs-dali/motivation-new.pdf}}
  \vspace{-1pt}
  \mycaption{Varying \#GPU and GPU generation for various DNNs}{This graph shows the percentage of total
    training time per epoch spent waiting for data 
    pre-processing for five different DNNs on 4 and 8 GPUs. Input data was completely
    cached, requiring only pre-processing
    before use. }% The data stall time can be
   %as high as 70\% of total training time for some DNNs.}
  \label{fig-motivation}
\end{figure}
