# Supplementary material for: Analyzing and Mitigating Data Stalls in DNN Training
Source: arXiv:2007.06775 source file (2021-01-19)
Supplement: Supplementary file 27 [file appendix_main.tex]

%%%%%%%%%%%%%%%%%%%%%%%%%%%%%%%%%%%%%%%%%%%%%%%%%%%%%%%%%%%%%%%%%%%%%%%%%%%%%%%%
% Template for USENIX papers.
%
%%%%%%%%%%%%%%%%%%%%%%%%%%%%%%%%%%%%%%%%%%%%%%%%%%%%%%%%%%%%%%%%%%%%%%%%%%%%%%%%

\documentclass[letterpaper,twocolumn,10pt]{article}
\usepackage{usenix2019_v3}

% to be able to draw some self-contained figs
\usepackage{tikz}
\usepackage{amsmath}
\usepackage{adjustbox}
\usepackage{amsthm}
\usepackage{caption}
\usepackage{changepage}
\usepackage{datetime}
\usepackage{enumitem}
\usepackage{graphicx}
\usepackage{framed}
\usepackage{hyperref}
\usepackage{multirow}
\usepackage{url}
\usepackage{verbatim} % For comment
\usepackage{xspace} % For xspace
\usepackage[normalem]{ulem}
\usepackage{booktabs,array}
\newcommand\redsout{\bgroup\markoverwith{\textcolor{red}{\rule[0.5ex]{2pt}{0.4pt}}}\ULon}
\usepackage{titling}
\definecolor{dgreen}{HTML}{228B22}
\usepackage{xcolor}
\usepackage{setspace}

\newlength\mylength 

 \hypersetup{
	colorlinks=true,
	linkcolor=blue,
	filecolor=blue,
	citecolor = red,      
	urlcolor=red,
}

\usepackage[font=large, position=bottom]{subfig}
\usepackage{comment}
\usepackage{mdframed}
\mdfdefinestyle{MyFrame}{%
	linecolor=black,
	outerlinewidth=2pt,
	%roundcorner=20pt,
	innertopmargin=4pt,
	innerbottommargin=4pt,
	innerrightmargin=4pt,
	innerleftmargin=4pt,
	leftmargin = 4pt,
	rightmargin = 4pt,
	align=center
	%backgroundcolor=gray!50!white}
}

\usepackage[skins]{tcolorbox}

\newtcolorbox{mybox}{enhanced, sharp corners=all,colback=white,
	colframe=gray,toprule=0pt,bottomrule=0pt,leftrule=1pt,rightrule=1pt,
	right=1pt, left=1pt, top=1pt, bottom=1pt, halign=center, valign=center,
	overlay={
		\draw[gray,line width=2pt] (frame.north west) -- ++(8.45cm,0pt);
		\draw[gray,line width=1pt] (frame.south east) -- ++(-8.45cm,0pt);
	}
}

\newlength{\seplinewidth}
\newlength{\seplinesep}
\setlength{\seplinewidth}{0.5mm}
\setlength{\seplinesep}{2mm}
\colorlet{sepline}{gray}

%\usepackage{sectsty}
%\subsubsectionfont{\fontsize{10}{11}\selectfont}

% Remove ACM reference format
%\settopmatter{printacmref=false, printfolios=true, printccs=false}

% removes running headers
%\newlength{\savecw}

\input{macros}

% notes
\usepackage{ifthen}
\newboolean{publicversion}
%\setboolean{publicversion}{true}
\setboolean{publicversion}{false}

\IfFileExists{intro-flag}
{
  \setboolean{publicversion}{True}
}
{}

\ifthenelse{\boolean{publicversion}}{
	\newcommand{\grumbler}[3]{}
}{
	\newcommand{\grumbler}[3]{\xspace\textcolor{#3}{\bf #1: #2}}
}

% The default list of authors is too long for headers}
%\renewcommand{\shortauthors}{J Mohan et al.}

\setlength{\droptitle}{-1cm}
\posttitle{\par\end{center}\vspace{-40pt}}

\usepackage[compact]{titlesec}
%\titlespacing{\section}{0pt}{3pt}{3pt}
%\titlespacing{\subsection}{0pt}{2pt}{0ex}
%\titlespacing{\subsubsection}{0pt}{0.5ex}{0ex}
\titleformat{\subsection}{\normalfont\fontsize{11}{15}\bfseries}{\thesubsection}{1em}{}
%-------------------------------------------------------------------------------
\begin{document}
%-------------------------------------------------------------------------------

%don't want date printed
\date{}

% make title bold and 14 pt font (Latex default is non-bold, 16 pt)
\title{\Large \bf 
%\sysname: Analyzing and Mitigating Data Stalls in DNN Training
Appendix \\ \sysname: Coordinated Caching and Pre-processing for DNN Training
}

\maketitle

%{
	%\hypersetup{linkcolor=black}
	\tableofcontents
%}
\vspace{3em}
\input{appendix-intro}
\input{appendix_analysis}
\input{appendix_tool}
\input{appendix_eval}
\input{appendix_pytorch}

%-------------------------------------------------------------------------------
\bibliographystyle{plain}
\bibliography{all}

%%%%%%%%%%%%%%%%%%%%%%%%%%%%%%%%%%%%%%%%%%%%%%%%%%%%%%%%%%%%%%%%%%%%%%%%%%%%%%%%
\end{document}
