# Supplementary material for: Analyzing and Mitigating Data Stalls in DNN Training
Source: arXiv:2007.06775 source file (2021-01-19)
Supplement: Supplementary file 28 [file appendix_toc.tex]

%{
	%\hypersetup{linkcolor=black}
	\tableofcontents
%}
