# Supplementary material for: Analyzing and Mitigating Data Stalls in DNN Training
Source: arXiv:2007.06775 source file (2021-01-19)
Supplement: Supplementary file 30 [file fig-eval-hp-macro.tex]

 \begin{figure*}[!tbh]
  \centering 

      \subfloat[HP search job on ImageNet 22k\label{fig-hp-imagenet}] {{\includegraphics[width=.44\linewidth]{graphs-dali/hp-imagenet22k.pdf} }}%
       \qquad
       \subfloat[HP search job on OpenImages\label{fig-hp-openimages}] {{\includegraphics[width=.44\linewidth]{graphs-dali/hp-openimages.pdf} }}%
      
         \mycaption{End-to-end evaluation}{The graphs compare the training throughput per job when 8 concurrent HP search jobs run in a node using the DALI \dl and \sysname}
  \label{fig-eval-hp-macro}

\end{figure*}
